# Supplementary material for: TNS: Terrain Traversability Mapping and Navigation System for Autonomous Excavators
Source: arXiv:2109.06250 source file (2022-05-05)
Supplement: Supplementary file 1 [file appendix_back.tex]

In this section, we add more details of our planning experimentation. We compare the success rate of planner using output traversability map from geometric-only method~\cite{geo1} and from the proposed \ours{}. We use 9 different scenarios, and each scenario is tested with same starting points and random goal position with more than 10 trials. We list the details of all scenarios in Table~\ref{tab:exp}.

\begin{table}[t]
\centering
\resizebox{\columnwidth}{!}{%
\begin{tabular}{lcc|cc}
  \toprule
Scenarios & Difficult Terrain & Obstacles & Geometric Method~\cite{geo1} (\%)  & TTM (\%)  \\ 
  \midrule
Case 1   & \checkmark &  \checkmark    & 40      & \textbf{60  } \\
Case 2   & \checkmark &  \checkmark    & 16.67      & \textbf{71.43  } \\
Case 3   & \checkmark &      & 50      & 50   \\
Case 4   & \checkmark &  \checkmark    & 50      & \textbf{100  } \\
Case 5   & &  \checkmark    & 20      & \textbf{100  } \\
Case 6   & \checkmark &  \checkmark      & 40      & \textbf{80  } \\
Case 7   & &  \checkmark      & 50      & 50   \\
Case 8   & & \checkmark     & 20      & \textbf{60  } \\
Case 9   & \checkmark &      & 20      & \textbf{60  } \\
  \midrule
Overall & \checkmark & \checkmark & 33.3   & \textbf{82.6  } \\
\bottomrule
\end{tabular}
}
\caption{\textbf{Success rate of planning in each scenario.} ``Difficult Terrain'' means the excavator have to traverse through or navigate around a rough region or water. ``Obstackes'' means there are obstacles in the environment.}
\label{tab:exp}
\vspace{-10pt}
\end{table}

% 4 More map output with baidu bag and rellis bag -- vis
